# Supplementary material for: Is the largest aqueous gold cluster a superatom complex? Electronic structure & optical response of the structurally determined Au146(pMBA)57
Source: arXiv:1707.00279 ancillary file (2017-07-02)
Supplement: Supplementary file 1 [file supp_mat_V1_small.pdf]

# Is the largest aqueous gold cluster a superatom complex? Electronic structure & optical response of the structurally determined $Au_{146}(pMBA)_{57}$.

**Xóchitl López-Lozano,**[a] **G. Plascencia-Villa,**[a] **G. Calero,**[b] **R.L.Whetten,**[*a] **and Hans-Christian Weissker**[*cd]

[a] Department of Physics & Astronomy, The University of Texas at San Antonio, One UTSA circle, 78249-0697 San Antonio, TX., USA

[b] Dpt. of Structural Biology, University of Pittsburg, Pittsburg, PA, USA

[c] Aix Marseille University, CNRS, CINaM UMR 7325, 13288, Marseille, France; Email: weissker@cinam.univ-mrs.fr

[d] European Theoretical Spectroscopy Facility, etsf.eu

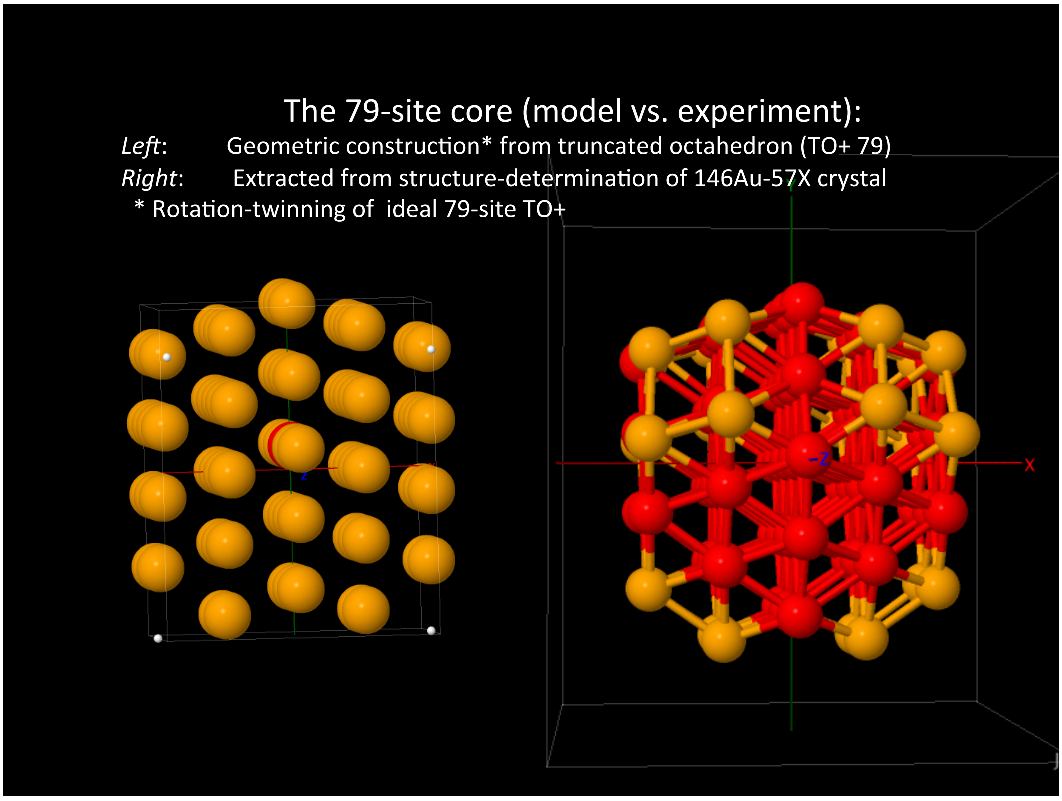


**Figure S1.** Visualization of the 78-site core that shows the twinned 79-atom truncated octohedron.

## Projection of orbitals onto spherical harmonics to obtain the angular-momentum-projected density of states (pDOS)

To obtain the angular-momentum-projected DOS, we follow Ref. 1 and calculate the projection coefficients

$$w_{i,l} = \sum_{m=-l}^{l} \int \rho^2 d\rho \left| \int d\Omega \, Y_{l,m}[\Omega] \, \psi(\mathbf{r}) \right|^2 = \sum_{m=-l}^{l} \sum_{n} |c_{nlm}|^2 \tag{1}$$

where $\psi_i$ are the Kohn-Sham wave functions from the octopus ground-state calculation, $Y_{l,m}$ the spherical harmonics, and the $c_{nlm}$ are the expansion coefficients

$$\psi(\rho, \phi, \theta) = \sum_{nlm} c_{nlm} R_{nlm}(\rho) Y_{lm}(\phi, \theta) \tag{2}$$

The integration was done up to a radius $R_{\text{cut}}$. For the present system, the result was found to be very insentitive to the choice of $R_{\text{cut}}$.

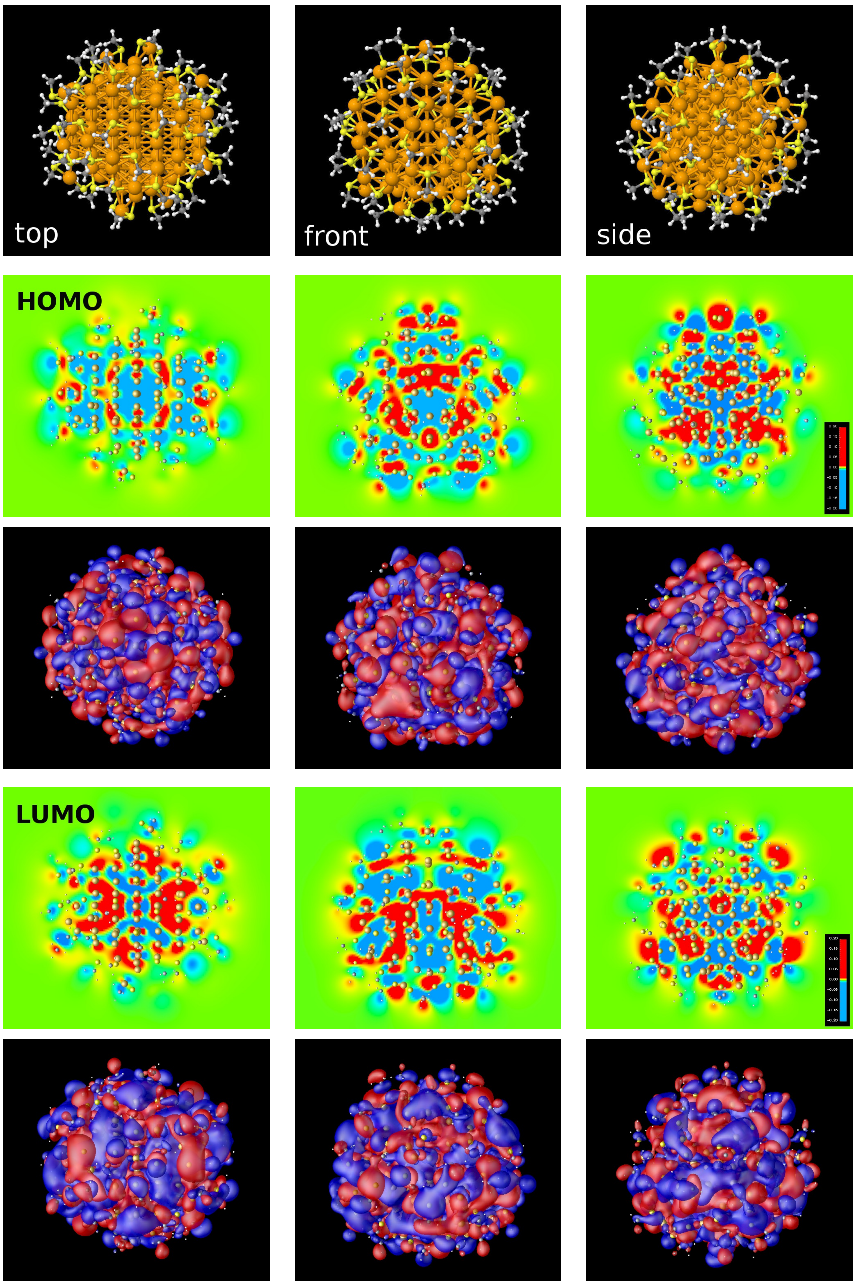


**Figure S2: Frontier orbitals of the $Au_{146}(SCH_3)_{57}$ cluster along with the geometry of the $R{=}CH_3$ model used in the calculation.** We show the geometry from the three different perspectives (top, front, side) which are then used for the presentation of the states. These are slice representations, cutting through the center of the cluster (blue – negative, red – positive), as well as isosurfaces of the same states (iso value 0.005 $Å^{-3}$). Note that the top isosurface view of HOMO and LUMO concerns the same states as shown in Fig. 2 of the article; the visual difference comes from the different iso values used. Slice representations of the full series of states around the HOMO-LUMO gap are shown in Fig. S3 of the the ESI.

Note that due to the symmetry, the top views of the slice representations have an *approximate* mirror symmetry at the center (representing the symmetry of the core), which is, however, broken in the periphery so that only the screw-like symmetry (180-degree rotation) remains, in accordance with the $C_2$ symmetry of the full system where the chiral character is introduced in the peripheral Au layer and the ligands. The front and side views for the slices through the center, by contrast, are mirror symmetric. However, this holds only for the slice views cutting through the center. Seen from outside, the system is not symmetric except for the two-fold rotation axis, as it is clearly seen in the isosurfaces.

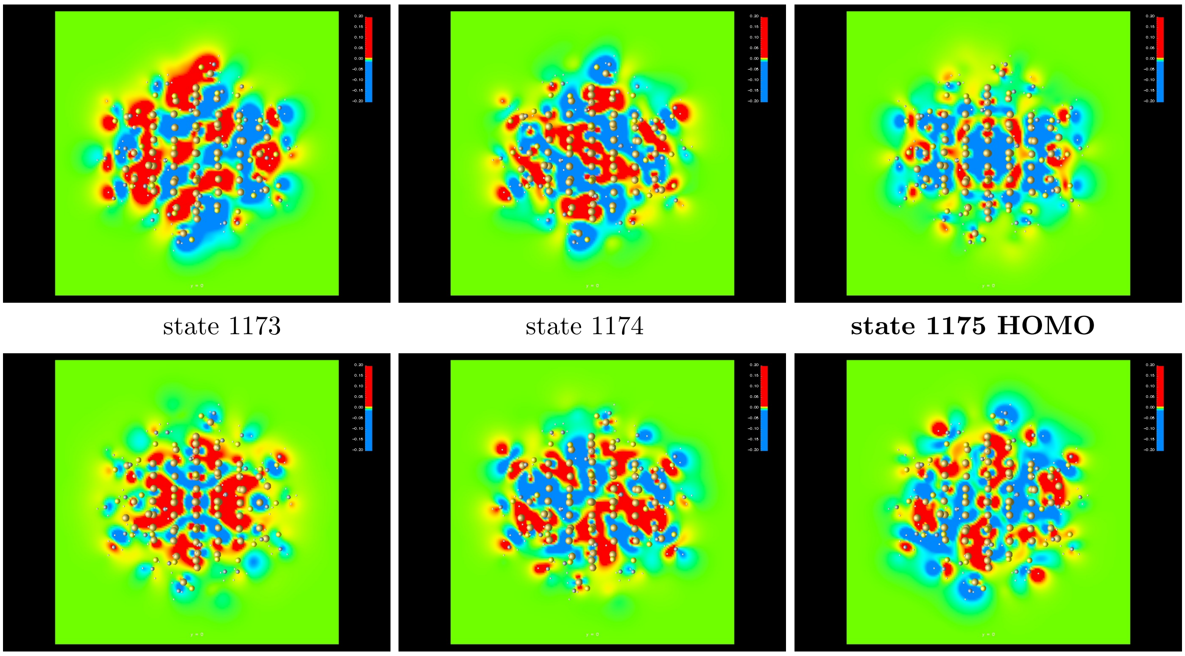

state 1173 | state 1174 | **state 1175 HOMO**

**state 1176 LUMO** | state 1177 | state 1178

**Figure S3.** Series of the wave functions of $Au_{146}(SCH_3)_{57}^{-3}$ around the HOMO-LUMO gap (sliced through the center (cutting through the center atom); top view, i.e., we are looking down the two-fold rotation axis.

• States 1174, 1175 = HOMO, 1176 = LUMO, and 1178 are symmetric under the 180 degree rotation around the symmetry axis, the other states ( 1173, 1177 ) are **antisymmetric**, i.e., they change sign under the two-fold rotation. The $C_2$ symmetry is clearly visible.

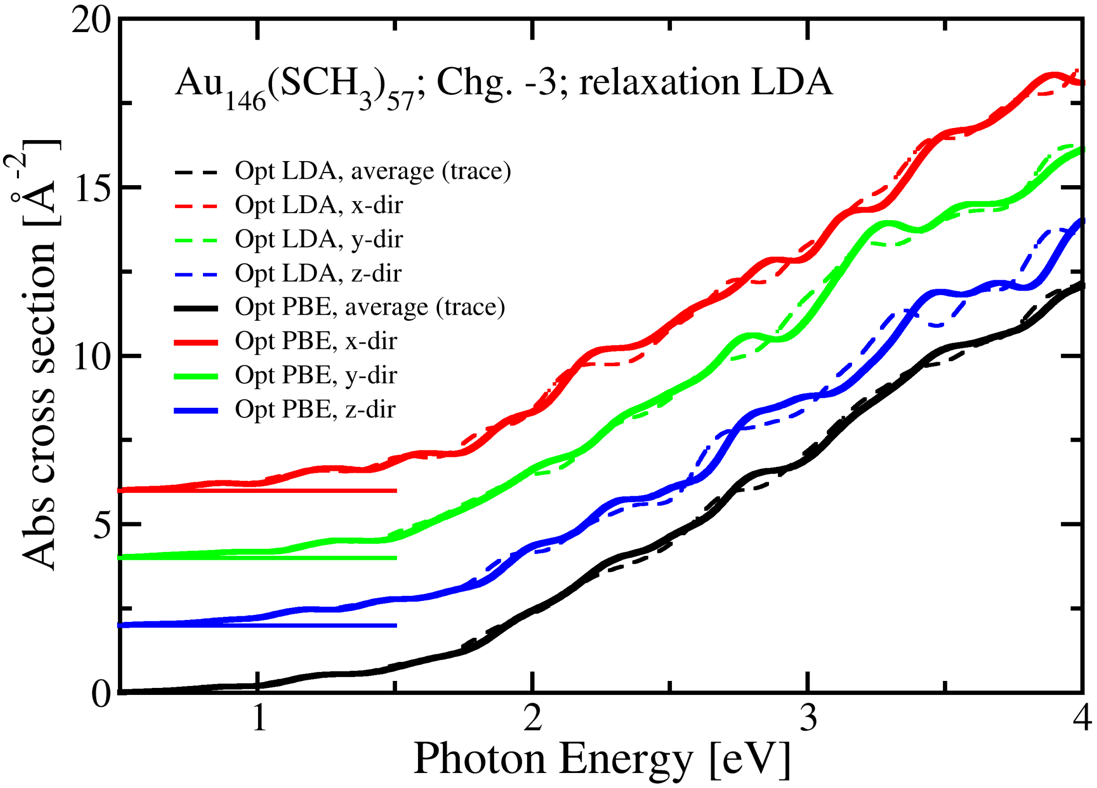


**Figure S4.** Comparison of spectra calculated using the LDA functional and the GGA functional PBE. Both calculations use the same structure, relaxed using LDA.

# References

[1] Michael Walter, Jaakko Akola, Olga Lopez-Acevedo, Pablo D. Jadzinsky, Guillermo Calero, Christopher J. Ackerson, Robert L. Whetten, Henrik Grönbeck, and Hannu Häkkinen. A unified view of ligand-protected gold clusters as superatom complexes. *Proceedings of the National Academy of Sciences*, 105(27):9157–9162, 2008.
